# Supplementary material for: EMaQ: Expected-Max Q-Learning Operator for Simple Yet Effective Offline and Online RL
Source: arXiv:2007.11091 source file (2021-01-13)
Supplement: Supplementary file 1 [file online_rl_appendix.tex]

\section{Online RL}
    \label{ap:online_rl}
    Combining strong off-policy RL methods with good exploration policies has the potential for producing highly sample-efficient online RL algorithms. Concretely, we refer to online RL as the setting where iteratively, a batch of $M$ environment steps with an exploration policy are interleaved with $K$ RL updates
    ~\citep{levine2020offline,matsushima2020deployment}.
    % ~\citep{levine2020offline}.
    
    \subsection{Challenge of Converting to Online RL}
        By design, our proposed method EMaQ, does a good job of remaining within the support of the provided training distribution (we also take our empirical results to be indicative of this). This however, is problematic for online RL which requires good exploration interleaved with good RL updates. While our initial results are promising for obtaining very sample-efficient policies, it is still a work in progress for us to understand how to make these algorithms more reliable.
    
    \subsection{Method}
        For our initial results with online RL, we designed an online policy as follows. First, we modify our autoregressive proposal distribution $\muas$ by dividing the logits of all softmaxes by $\tau > 1$. This has the effect of smoothing the $\muas$ distribution, increasing the probability of sampling actions from the low-density regions and the boundaries of the support. Given this online proposal distribution, we need a criteria by which to choose amongst sampled actions. We use a UCB-style exploration criterion as follows:
        \begin{align}
            Q^{\mbox{explore}}(s,a) = \mbox{mean}\Big(\{Q_i(s,a)\}_K\Big) + \beta \cdot \mbox{std}\Big(\{Q_i(s,a)\}_K\Big)
        \end{align}
        Given $N$ sampled actions from the modified proposal distribution, we take the action with highest $Q^{\mbox{explore}}$. In our experiments thus far we have used $\lambda = 1.0$ and focused our hyperprameter search on the value of the softmax temperature $\tau$.
        % We briefly explored two avenues for designing exploration policies to be interleaved with EMaQ updates.
        % \paragraph{Using Max Q for Exploration}
        
        % \paragraph{UCB-Style Exploration}
        
        We have not yet tested exploration methods such as 1) using the max of the Q functions, and 2) in each episode randomly choosing one of the Q functions and acting greedily according to that Q function.
        
    \subsection{Results for Online EMaQ versus SAC}
        In this section, we benchmark the performances of online EMaQ against SAC baselines. For fairness of comparisons, we also ran SAC with similar sweeps over different collection batch sizes and number of Q-function ensembles. For SAC, we used the entropy-constrained automatic tuning of temperature variable, while for EMaQ we swept the temperatures and used a fixed bin size of 40, 8 Q-function ensembles and $N=200$.
        Figures \ref{fig:all_batch_1} and \ref{fig:all_batch_50K} present the results for all hyperparameter settings, for SAC and EMaQ, in the batch size $1$ and batch size $50K$ settings respectively.
        % Figures~\ref{fig:online_emaq_1_40} and~\ref{fig:online_emaq_50k_40} show side-by-side comparisons of EMaQ and SAC.
        \textbf{In the fully online setting, EMaQ is already competitive with SAC, and more excitingly, in the deployment-efficient setting, EMaQ can outperform SAC.}
        % Figures~\ref{fig:online_sac_2_qs} and~\ref{fig:online_sac_8_qs} show ablation results for SAC.
    
        % \begin{figure}[h]
        %     \centering
        %     \includegraphics[width=\textwidth]{figs/online_rl.png}
        %     \caption{Caption}
        %     \label{fig:Online RL Results}
        % \end{figure}
        
    \begin{figure}
        \centering
        
        \begin{subfigure}{\textwidth}
            \centering
            \includegraphics[width=\textwidth]{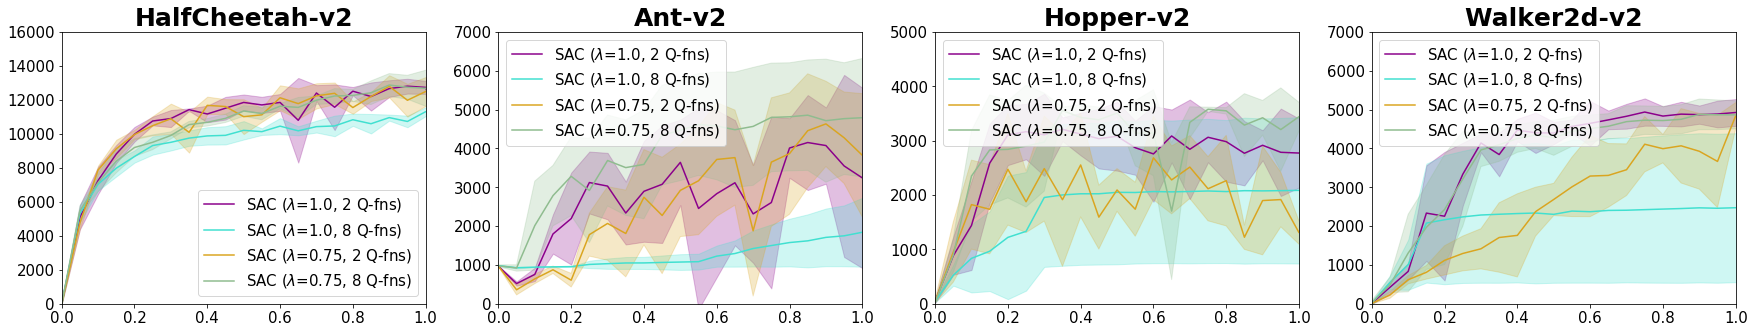}
            \caption{SAC batch 1 results}
        \end{subfigure}
        \begin{subfigure}{\textwidth}
            \centering
            \includegraphics[width=\textwidth]{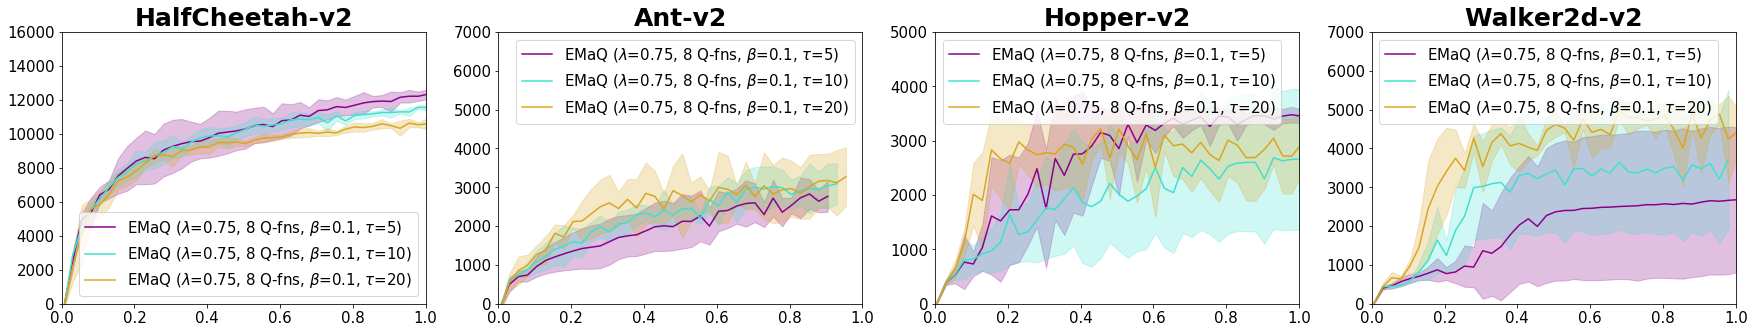}
            \caption{EMaQ batch 1 results}
        \end{subfigure}
        
        \caption{All results for batch size 1}
        \label{fig:all_batch_1}
    \end{figure}
    
    \begin{figure}
        \centering
        
        \begin{subfigure}{\textwidth}
            \centering
            \includegraphics[width=\textwidth]{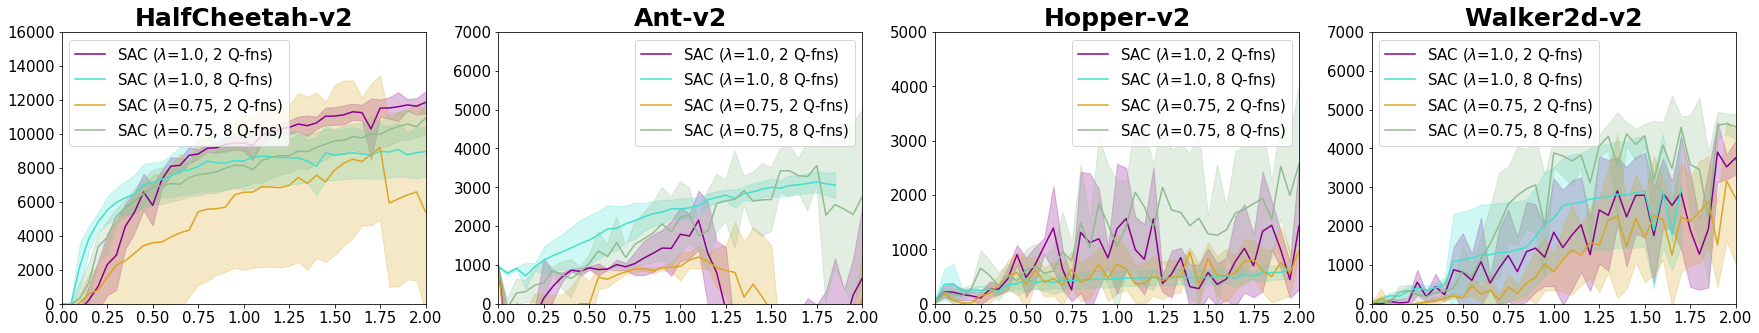}
            \caption{SAC batch 50K results}
        \end{subfigure}
        \begin{subfigure}{\textwidth}
            \centering
            \includegraphics[width=\textwidth]{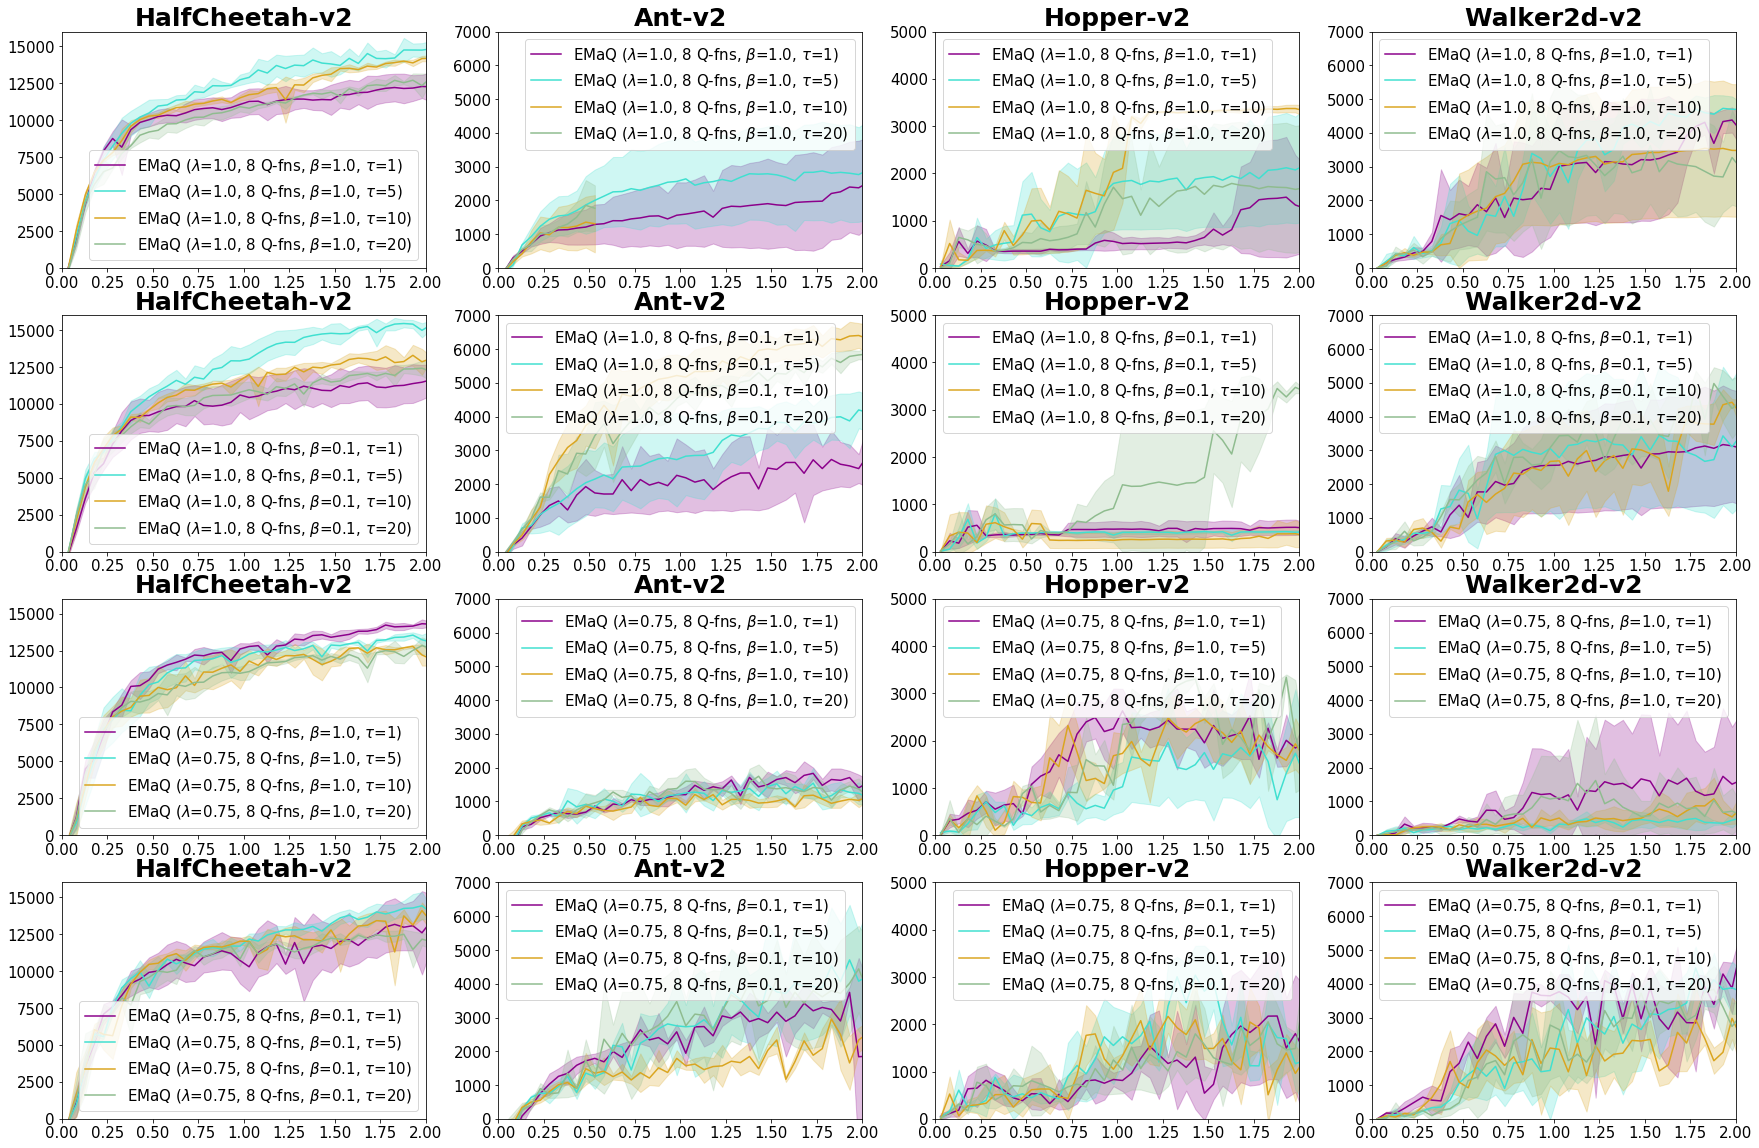}
            \caption{EMaQ batch 50K results}
        \end{subfigure}
        
        \caption{All results for batch size 50K}
        \label{fig:all_batch_50K}
    \end{figure}
